# Supplementary material for: Multilevel adaptive sparse Leja approximations for Bayesian inverse problems
Source: arXiv:1904.12204 source file (2019-05-07)
Supplement: Supplementary file 1 [file appendix.tex]

\appendix
\section{One-dimensional approximation operators setup}
\label{sec:sg_setup}
\subsection{Interpolation and quadrature operators} \label{subsec:operators}
In this paper, the univariate operators $\mathcal{U}^{i}[f^i]$ used to construct the sparse grid approximations are identical for all input directions $i$.
Hence we omit the superscript and use the notation $\mathcal{U}[f^i]$ and $\mathcal{U}_k[f^i]$, respectively.
We consider two types of univariate approximation operators, interpolation and quadrature, on which we build our proposed multilevel approach.

A popular interpolation strategy is \emph{Lagrange interpolation} (see, e.g., \cite{Fa18, Fo13, HajiAlietal:2016, NJ14, TJWG:2015}), which we use in this work.
Let $N_k$ denote the number of interpolation points at level $k$.
The corresponding one dimensional Lagrange interpolation operator reads
\begin{equation} \label{eq:interp_1D} 
f^i(\theta) \approx \mathcal{U}^{\mathrm{in}}_k[f^i](\theta) :=\sum_{n = 1} ^ {N_k} f^i(\theta_n) L_n(\theta),
\end{equation}
where $f^i \in C^0(X_i)$, $\{\theta_n\}_{n=1}^{N_k}$ are the interpolation knots at level $k$ and $L_n(\theta)$ are canonical Lagrange polynomials of degree $n - 1$ satisfying $L_n(\theta_m) = \delta_{nm}$, where $\delta_{nm}$ is Kronecker's delta function. 
For improved numerical stability, we implement \cref{eq:interp_1D} in terms of the first form of the \emph{barycentric formula} (see, e.g., \cite{BT04}).

In addition, we also employ \emph{interpolatory quadrature operators} defined  as 
\begin{equation*}
\int_{D}f^i(\theta) w(\theta) d \theta \approx \mathcal{U}^{\mathrm{qu}}_k[f^i] := \sum_{n = 1} ^ {N_k} f^i(\theta_n)w_n,
\end{equation*}
where $f^i$ is an integrable function, $\{\theta_n\}_{n=1}^{N_k}$ are the quadrature nodes at level $k$ and $\{w_n\}_{n=1}^{N_k}$ are the associated quadrature weights.
The quadrature weights are computed as follows.
Let $\psi_p$, $p = 0, \ldots, N_k - 1$ denote a family of polynomials of degree $p$ \emph{orthonormal} w.r.t. the weight function $w$, i.e.
\begin{equation*}
\left\langle \psi_p, \psi_q \right\rangle_w := \int_{D}\psi_p(\theta) \psi_q(\theta) w(\theta) d \theta = \delta_{pq}.
\end{equation*}
Defining the matrix $\Psi \in \mathbb{R}^{N_k \times N_k}$ with entries $\Psi_{i,j} = \psi_{i - 1}(\theta_j)$, $i, j = 1, 2, \ldots, N_k$, the first row of $\Psi^{-1}$ yields the quadrature weights $\{w_n\}_{n=1}^{N_k}$ due to the orthonormality of the polynomials $\psi_p$ (see, e.g., \cite{NJ14}).
Note that since $w$ is a univariate probability density function, $\{w_n\}_{n=1}^{N_k}$ are normalized, i.e., $\sum_{n=1}^{N_k} w_n = 1$. 

\begin{remark} \label{re:remark_nestedness}
If $\{\theta_n\}_{n=1}^{N_{k - 1}}$ is a subset of $\{\theta_n\}_{n=1}^{N_k}$, i.e., the point sets are nested, the linearity of the one dimensional operators implies that the evaluations used to determine $\mathcal{U}_{k - 1}[f^i]$ can be reused when computing $\mathcal{U}_{k}[f^i]$. 
In other words, $\mathcal{U}_{k}[f^i]$ needs to be evaluated only on the set difference $\{\theta_n\}_{n=1}^{N_k} \setminus \{\theta_n\}_{n=1}^{N_{k - 1}} = \{\theta_n\}_{n=N_{k - 1} + 1}^{N_k}$.
\end{remark}

% \begin{remark} \label{re:remark_indep}
% The tensorized construction of $\boldsymbol{\mathcal{U}}_{\mathcal{K}}[f^{\boldsymbol{N_\sto}}]$ implies that 
% the underlying parameter space needs to have a tensor structure. 
% In our setting this means that the underlying probability density should be of product form.
% That is, all random variables used in the approximation are stochastically independent.
% \end{remark}

\subsection{Weighted (L)-Leja sequences} \label{subsec:weighted_leja}
%The popular point sets for interpolation and quadrature are Gauss points, such as Gauss-Legendre or Gauss-Hermite \cite{Xi10}, and Clenshaw-Curtis points \cite{CC60}. 
%However, these choices are limited to specific probability densities. 
%Gauss-Hermite points are associated with Gaussian densities, and Gauss-Legendre and Clenshaw-Curtis points are used for uniform densities. 
%Moreover, although these points have excellent approximation properties, their number usually increases exponentially with the level. 
%In addition, only some, e.g. Clenshaw-Curtis points, are nested (\cref{re:remark_nestedness}). 

In this work, we want a point set that allows interpolation and quadrature operators to be defined for arbitrary probability densities.
Moreover, we also want a point set that
\begin{itemize}
\item is nested: so that we can reuse computations from previous levels,
\item  grows slowly with the level: so that the total number of grid points per level is not large,
\item leads to accurate approximations.
\end{itemize}
To this end, we employ weighted (L)-Leja sequence (see, e.g., \cite{GO16, NJ14}).

Given the weight function $w: X_i \rightarrow \mathbb{R}$, \emph{weighted (L)-Leja sequences} are constructed recursively as follows:
\begin{equation}\label{eq:weighted_leja_points}
\begin{split}
& \theta_1 = \underset{\theta \in X_i}{\mathrm{argmax}}{\ |w(\theta)|}, \\
\ & \theta_n = \underset{\theta \in X_i}{\mathrm{argmax}} \ |w(\theta)\prod_{m=1}^{n-1}(\theta - \theta_m)|, \quad n = 2, 3, \ldots
\end{split}
\end{equation}
When $w$ is the standard uniform density with support $[0, 1]$, we choose $\theta_1 = 0.5$.
Note that the above point sequence is in general not uniquely defined, because \cref{eq:weighted_leja_points} might have multiple optimums.
In that case we simply pick one of the maximizers.
%We illustrate the weighted (L)-Leja construction \cref{eq:weighted_leja_points} in  \cref{fig:weighted_leja_constr}.
%On the left-hand side we depict the (L)-Leja points for the uniform density on $D=[0, 1]$ using $\theta_1 = 0.5$. 
%In the right plot we depict the points for the standard Gaussian density on $D=\mathbb{R}$ using $\theta_1 = 0$.  

The construction \cref{eq:weighted_leja_points} indicates that weighted (L)-Leja points form an interpolatory sequence, i.e., only one extra point is needed to increase the interpolation degree by one.
Recall that $N_k$ denotes the number of weighted (L)-Leja points at level $k$.
In this paper we employ $N_k = 1$ for interpolation. 
For quadrature, $N_1 = 1$ and $N_k = 2k - 1, \quad k \geq 2$, that is, we add two extra points for all levels greater than $2$.
This is because when the weight function $w$ is symmetric, adding only one (L)-Leja point at a time will lead to a zero quadrature weight at level $k=2$, causing the adaptive algorithm employed in this paper to stop prematurely.
%\begin{figure}[htbp]
%  \centering
%  \includegraphics[width=1.0\textwidth]{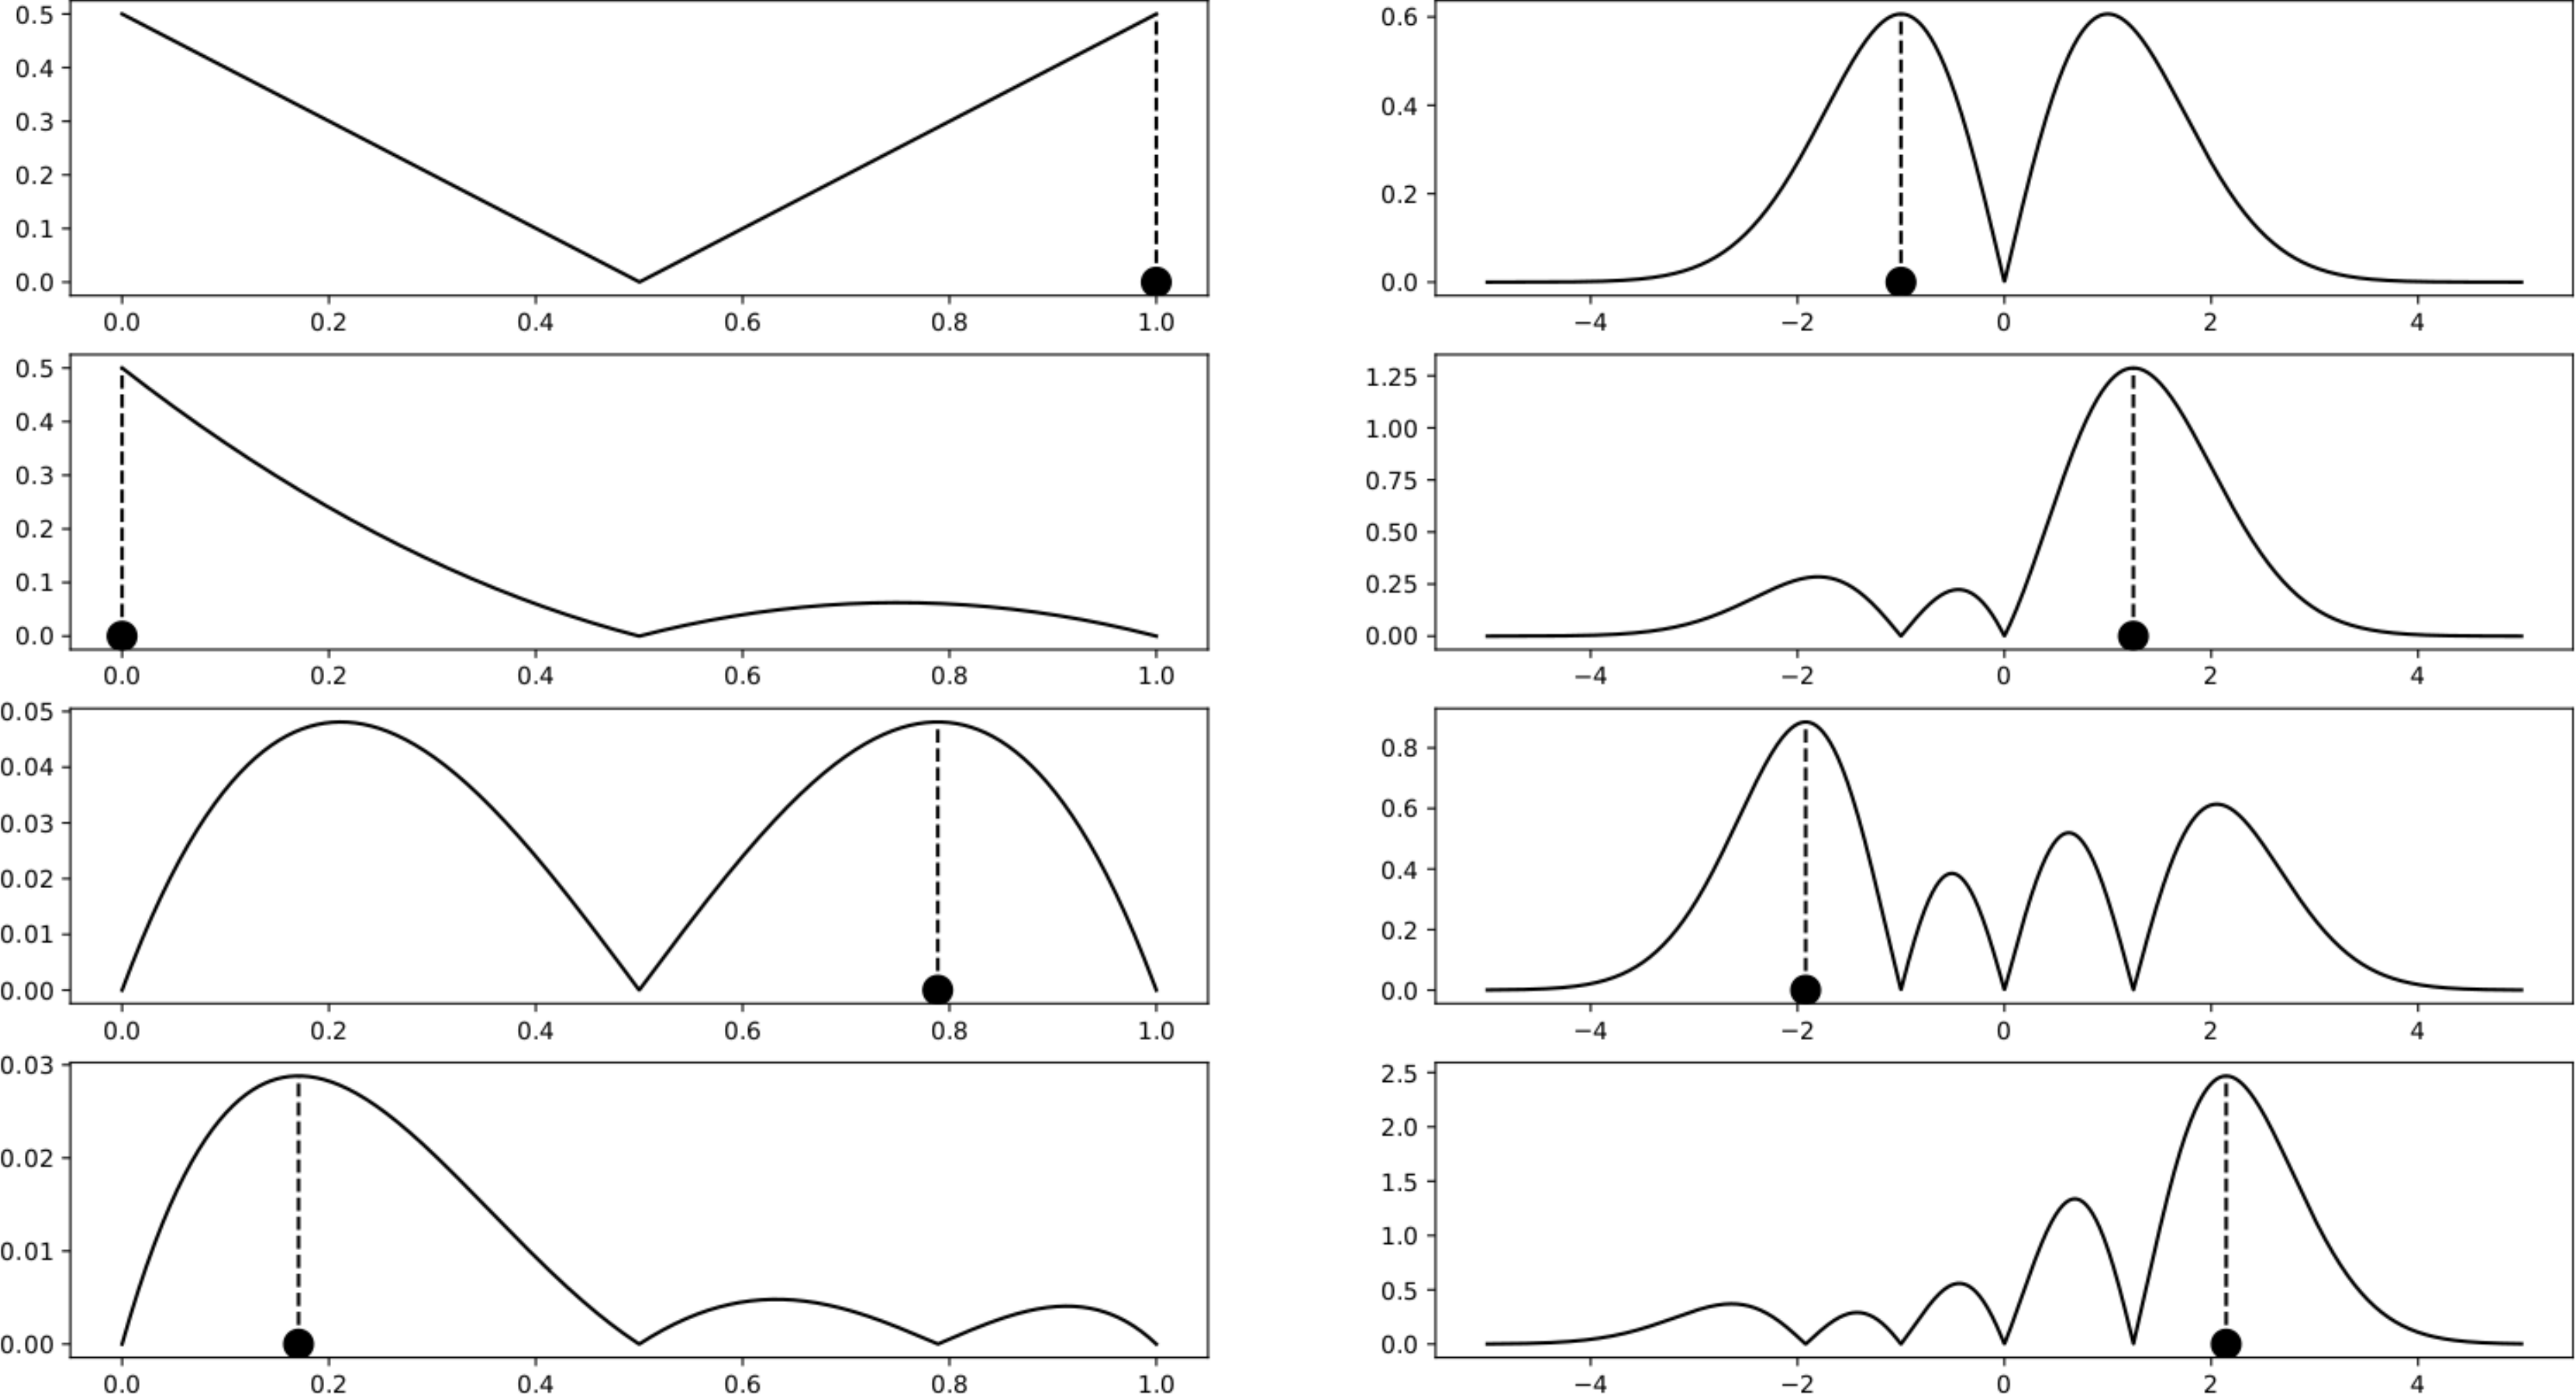}
%  \caption{Weighted (L)-Leja sequence of points.
%  	From top to bottom we depict the function $|w(\theta)\prod_{m=1}^{n-1}(\theta - \theta_m)|$ and the corresponding Leja points (dots) for $n = 2, \ldots, 5$. 
%  	On the left-hand side $D=[0, 1]$, $w \equiv 1$ and $\theta_1= 0.5$. 
%  	In the right part $D=\mathbb{R}$, $w(\theta) = \frac{1}{\sqrt{2\pi}}\exp{(-\theta^2/2)}$ and $\theta_1 = 0$.}
%  \label{fig:weighted_leja_constr}
%\end{figure}
More details on (L)-Leja points and their properties can be found in \cite{GO16, NJ14} and the references therein.

\section{Dimension-adaptive algorithms}
\subsection{$L^2$ norm of surpluses for adaptive sparse grid interpolation} \label{subsec:l2_norm}
To assess $\| \boldsymbol{\Delta}^{\mathrm{in}}_{\boldsymbol{k}}[f^{\boldsymbol{N_\sto}}] \|_{L^2}$ we proceed analogously to \cite{Fa18b}.
Recall that for interpolation the number of points corresponding to $\boldsymbol{k}$ is ${N_{\boldsymbol{k}}} := \prod_{i=1}^{N_\sto} k_i$ (see \cref{subsec:weighted_leja}). 
This leads to a total multivariate interpolation degree $\boldsymbol{I}_{\boldsymbol{k}} = (k_1 - 1, k_2 - 1, \ldots, k_d - 1)$ with cardinality $N_{\boldsymbol{k}}$.
Initially, we perform a transformation from the Lagrange basis to an equivalent basis orthonormal of the same total degree, i.e.,
\begin{equation}\label{eq:spectral_to_interp_fg}
\boldsymbol{\mathcal{U}}^{\mathrm{in}}_{\boldsymbol{k}}[f^{\boldsymbol{N_\sto}}](\boldsymbol{\theta}) = \sum_{\boldsymbol{p} = \boldsymbol{0}}^{\boldsymbol{I}_{\boldsymbol{k}}} \gamma_{\boldsymbol{p}} \boldsymbol{\Psi}_{\boldsymbol{p}}(\boldsymbol{\theta}),
\end{equation}
where $\boldsymbol{\Psi}_{\boldsymbol{p}}(\boldsymbol{\theta}) := \prod_{i=1}^{N_\sto}\Psi_{p_i}(\theta_i)$ are the orthonormal polynomials and $\gamma_{\boldsymbol{p}}$ are the corresponding spectral coefficients, i.e., the coordinates in the orthonormal basis.
We obtain the surplus spectral coefficients associated to $\boldsymbol{\Delta}^{\mathrm{in}}_{\boldsymbol{k}}[f^{\boldsymbol{N_\sto}}]$ as
\begin{equation} \label{eq:spectral_coeff_delta}
\Delta \gamma_{\boldsymbol{p}} = \sum_{\boldsymbol{z} \in \{0, 1\}^{N_\sto}} (-1)^{|\boldsymbol{z}|_1} \gamma_{\boldsymbol{p} - \boldsymbol{z}},
\end{equation}
where $\Delta \gamma_{\boldsymbol{0}} := \gamma_{\boldsymbol{0}}$.
We assess $\{\gamma_{\boldsymbol{p}}\}_{\boldsymbol{p} = \boldsymbol{0}}^{\boldsymbol{I}_{\boldsymbol{k}}}$ by solving $\sum_{\boldsymbol{p} = \boldsymbol{0}}^{\boldsymbol{I}_{\boldsymbol{k}}} \gamma_{\boldsymbol{p}} \boldsymbol{\Psi}_{\boldsymbol{p}}(\boldsymbol{\theta}_n) = \boldsymbol{\mathcal{U}}^{\mathrm{in}}_{\boldsymbol{k}}[f^{\boldsymbol{N_\sto}}](\boldsymbol{\theta}_n)$ for all weighted (L)-Leja points $\boldsymbol{\theta}_n$ corresponding to $\boldsymbol{\mathcal{U}}^{\mathrm{in}}_{\boldsymbol{k}}[f^{\boldsymbol{N_\sto}}]$. 
This amounts to solving a linear system of equations for which we employ the LAPACK routine $\_$gesv (see \cite{St06}).
Afterwards, we compute $\Delta \gamma_{\boldsymbol{p}}$ via \cref{eq:spectral_coeff_delta}.

Due to the orthonormality of the basis polynomials $\{\boldsymbol{\Psi}_{\boldsymbol{p}}\}_{\boldsymbol{p} = \boldsymbol{0}}^{\boldsymbol{I}_{\boldsymbol{k}}}$, we have
\begin{equation} \label{eq:l2_norm_spectral}
\| \boldsymbol{\Delta}_{\boldsymbol{k}}^{\mathrm{in}}[f^{\boldsymbol{N_\sto}}] \|_{L^2}^2 = \sum_{\boldsymbol{p} = \boldsymbol{0}}^{\boldsymbol{I}_{\boldsymbol{k}}} \Delta \gamma_{\boldsymbol{p}}^2.
\end{equation}
In \cite[Chapter 5.3]{Xi10} it was shown that the mean and variance can be computed analytically from the spectral coefficients. 
To this end, the first term in \cref{eq:l2_norm_spectral} represents the expectation contribution, which is usually small (see, e.g., \cite{Wi16}), while the terms $\gamma_{j \geq 2}^2$ are local contributions to the variance. 
Hence, using the $L^2$-norm of the surplus in the standard indicator \cref{eq:adapt_interp_std} means that the refinement process is driven by stochastic information, which is desirable in our context.

\subsection{Standard dimension-adaptive algorithm} \label{subsec:std_adapt_algo}
\begin{algorithm}
\caption{Standard dimension-adaptive sparse approximation}\label{algo:std_adapt}
\begin{algorithmic}[1]
\Procedure{StdAdaptivity}{$tol^{\mathrm{op}}, K_{\mathrm{max}}^{\mathrm{op}}, f^{\boldsymbol{N_\sto}}(\boldsymbol{\theta}), \pi(\boldsymbol{\theta}), s^{\mathrm{op}}(\cdot)$}
\State $\boldsymbol{1} = (1, 1, \ldots, 1), \quad \mathcal{O} = \emptyset, \quad \mathcal{A} = \{\boldsymbol{1}\}$
\State Compute $\epsilon(\boldsymbol{1}) =  s^{\mathrm{op}}(\boldsymbol{\Delta}_{\boldsymbol{1}}^{\mathrm{op}}[f^{\boldsymbol{N_\sto}}])/\delta N_{\boldsymbol{1}} =  s^{\mathrm{op}}(\boldsymbol{\Delta}_{\boldsymbol{1}}^{\mathrm{op}}[f^{\boldsymbol{N_\sto}}])$ based on $\pi(\boldsymbol{\theta})$
\State $\rho = \epsilon(\boldsymbol{1})$
\While{$\rho \geq tol^{\mathrm{op}}$ or $\mathcal{A} \neq \emptyset$ or $\max(\mathcal{K}) \leq K_{\mathrm{max}}^{\mathrm{op}}$}
\State Select $\boldsymbol{k}$ from $\mathcal{A}$ with the largest $\epsilon(\boldsymbol{k})$
\State $\mathcal{A} = \mathcal{A} \setminus \{\boldsymbol{k}\}, \quad \mathcal{O} = \mathcal{O} \cup \{\boldsymbol{k}\}$
\State $\rho = \rho - \epsilon(\boldsymbol{k})$
\For{$i\gets 1, N_\sto$}
\State $\boldsymbol{r} = \boldsymbol{k} + \boldsymbol{e}_i$
\If{$\boldsymbol{r} - \boldsymbol{e}_q \in \mathcal{O}$ for all $q = 1, 2, \ldots, N_\sto$}
\State $\mathcal{A} = \mathcal{A} \cup \{\boldsymbol{r}\}$
\State Compute $\epsilon(\boldsymbol{r}) =  s^{\mathrm{op}}(\boldsymbol{\Delta}_{\boldsymbol{r}}^{\mathrm{op}}[f^{\boldsymbol{N_\sto}}])/\delta N_{\boldsymbol{r}}$ based on $\pi(\boldsymbol{\theta})$
\State $\rho = \rho + \epsilon(\boldsymbol{r})$
\EndIf
\EndFor
\EndWhile
\State $\mathcal{K} = \mathcal{O} \cup \mathcal{A}$
\State \Return $\mathcal{K}$ 
\EndProcedure
\end{algorithmic}
\end{algorithm}
The inputs of the standard dimension-adaptive algorithm for interpolation and quadrature are the user-defined tolerance $tol^{\mathrm{op}}$, the maximum attainable sparse grid level $K_{\mathrm{max}}^{\mathrm{op}}$, the multivariate function $f^{\boldsymbol{N_\sto}}(\boldsymbol{\theta})$, and the density $\pi(\boldsymbol{\theta})$ w.r.t. which the approximation is computed, i.e., the weight w.r.t. which the (L)-Leja sequence is constructed.
The last input parameter is the numerator of the standard error indicator \cref{eq:std_error_indicator}, $s^{\mathrm{op}}(\cdot)$. 
Recall that to construct the underlying sparse grid approximation, $\pi(\boldsymbol{\theta})$ needs to be separable.

\subsection{Directional variance dimension-adaptive sparse interpolation}\label{subsec:dir_var_adapt_algo}
In the following, we summarize the directional-variance-enhanced dimension-adaptive algorithm for sparse grid interpolation.
The inputs are the user-defined global interpolation tolerance $tol^{\mathrm{in}}$, the maximal attainable level $K_{\mathrm{max}}^{\mathrm{in}}$, the multivariate function $f^{\boldsymbol{N_\sto}}(\boldsymbol{\theta})$, and the density $\pi(\boldsymbol{\theta})$ w.r.t. which the sparse interpolation is performed and the associated weighted (L)-Leja points are constructed.
The last input is $\boldsymbol{\tau}^{\mathrm{in}}$, comprising the $N_\sto$ directional tolerances, i.e., $\boldsymbol{\tau}^{\mathrm{in}} := (\tau_1^2, \tau_2^2, \ldots, \tau_{N_\sto}^2)$. 

The directional variances are computed in steps 7 -- 8 for the first adaptive steps and in steps 22 -- 23 for the remaining steps. 
In addition, the directional variance-based approach ends also if all directional variances fall below the tolerances $\boldsymbol{\tau}^{\mathrm{in}}$, i.e., $\mathcal{V}_{\mathcal{A}}^{\mathrm{tot}} \geq \boldsymbol{\tau}^{\mathrm{in}}$.
All other steps are as in \cref{algo:std_adapt}.
\begin{algorithm}
\caption{Directional variance dimension-adaptive sparse interpolation}\label{algo:mod_adapt}
\begin{algorithmic}[1]
\Procedure{DirVarAdaptivity}{$tol^{\mathrm{in}}, K_{\mathrm{max}}^{\mathrm{in}}, f^{\boldsymbol{N_\sto}}(\boldsymbol{\theta}), \pi(\boldsymbol{\theta}), \boldsymbol{\tau}^{\mathrm{in}}$}
\State $\boldsymbol{1} = (1, 1, \ldots, 1), \quad \mathcal{O} = \emptyset, \quad \mathcal{A} = \{\boldsymbol{1}\}$
\State $\mathcal{V}_{\mathcal{A}}^{\mathrm{tot}} = \emptyset$ \label{new_step_1}
\State Compute $\epsilon(\boldsymbol{1})= \| \boldsymbol{\Delta}_{\boldsymbol{1}}^{\mathrm{in}}[f^{\boldsymbol{N_\sto}}] \|_{L^2}$ based on $\pi(\boldsymbol{\theta})$ 
\State $\rho = \epsilon(\boldsymbol{1})$
\For{$i\gets 1, N_\sto$}
\State Compute $\Delta V_{\mathcal{A}}^{i, \mathrm{tot}}$ \label{new_step_2}
\State $\mathcal{V}_{\mathcal{A}}^{\mathrm{tot}} = \mathcal{V}_{\mathcal{A}}^{\mathrm{tot}} \cup \Delta V_{\mathcal{A}}^{i, \mathrm{tot}}$ \label{new_step_3}
\EndFor
\While{$\rho \geq tol^{\mathrm{in}}$ or $\mathcal{V}_{\mathcal{A}}^{\mathrm{tot}} \geq \boldsymbol{\tau}^{\mathrm{in}}$ or $\mathcal{A} \neq \emptyset$ or $\max(\mathcal{K}) \leq K_{\mathrm{max}}^{\mathrm{in}}$} \label{while_step}
\State Select $\boldsymbol{k}$ from $\mathcal{A}$ with the largest $\epsilon(\boldsymbol{k})$
\State $\mathcal{A} = \mathcal{A} \setminus \{\boldsymbol{k}\}, \quad \mathcal{O} = \mathcal{O} \cup \{\boldsymbol{k}\}$
\State $\rho = \rho - \epsilon(\boldsymbol{k})$
\State $\mathcal{V}_{\mathcal{A}}^{\mathrm{tot}} = \emptyset$ \label{new_step_4}
\For{$i\gets 1, N_\sto$}
\State $\boldsymbol{r} = \boldsymbol{k} + \boldsymbol{e}_i$
\If{$\boldsymbol{r} - \boldsymbol{e}_q \in \mathcal{O}$ for all $q = 1, 2, \ldots, N_\sto$}
\State $\mathcal{A} = \mathcal{A} \cup \{\boldsymbol{r}\}$ 
\State Compute $\epsilon(\boldsymbol{r}) =  \| \boldsymbol{\Delta}_{\boldsymbol{r}}^{\mathrm{in}}[f^{\boldsymbol{N_\sto}}] \|_{L^2}/\delta N_{\boldsymbol{r}}$ based on $\pi(\boldsymbol{\theta})$
\State $\rho = \rho + \epsilon(\boldsymbol{r})$
\EndIf
\State Compute $\Delta V_{\mathcal{A}}^{i, \mathrm{tot}}$ \label{new_step_5}
\State $\mathcal{V}_{\mathcal{A}}^{\mathrm{tot}} = \mathcal{V}_{\mathcal{A}}^{\mathrm{tot}} \cup \Delta V_{\mathcal{A}}^{i, \mathrm{tot}}$ \label{new_step_6}
\EndFor
\EndWhile
\State $\mathcal{K} = \mathcal{O} \cup \mathcal{A}$
\State \Return $\mathcal{K}$ 
\EndProcedure
\end{algorithmic}
\end{algorithm}
